# Supplementary material for: Robust and Efficient High-dimensional Quantum State Tomography
Source: arXiv:2010.00632 source file (2021-03-11)
Supplement: Supplementary file 1 [file SGQT_with_Qudits__Supplemental_Material.pdf]

# Robust and Efficient High-dimensional Quantum State Tomography: supplemental material

Markus Rambach,<sup>1,2,\*</sup> Mahdi Qaryan,<sup>1,2</sup> Michael Kewming,<sup>1,2</sup>  
Christopher Ferrie,<sup>3</sup> Andrew G. White,<sup>1,2</sup> and Jacqueline Romero<sup>1,2,†</sup>

<sup>1</sup>*Australian Research Council Centre of Excellence for Engineered Quantum Systems*

<sup>2</sup>*School of Mathematics and Physics, University of Queensland, QLD 4072, Australia*

<sup>3</sup>*Centre for Quantum Software and Information,  
University of Technology Sydney, NSW 2007, Australia*

(Dated: January 12, 2021)

## S1. HYPERPARAMETERS

The self-guided tomography algorithm operates based on an iterative optimisation technique called simultaneous perturbation stochastic approximation [1]. Regardless of the dimension  $d$  of the system, at every iteration, self-guided tomography calls two states  $|\sigma_{\pm}\rangle = |\sigma_k \pm \beta_k \Delta_k\rangle$  in relative to a randomly chosen direction  $(\Delta_k)_j \in \{1, -1, i, -i\}$  and measures the degree of their overlap with the unknown state  $|\psi\rangle$ . This provides an unbiased estimation of the gradient function that eventually leads to the best direction towards  $|\psi\rangle$ .

For each iteration, self-guided tomography calculates two functions ( $\alpha_k$  and  $\beta_k$ ) to decrease the upcoming step size. Both functions simultaneously control the size as well as the rate with which the steps become smaller between iterations. Their parameters are user defined and follow

$$\alpha_k = \frac{a}{(k+1+A)^s}, \quad \beta_k = \frac{b}{(k+1)^t}, \quad (1)$$

where  $k$  is the iteration number and  $a$ ,  $A$ ,  $b$ ,  $s$ , and  $t$  are the hyperparameters. Although the numerical studies on a variety of different problems can approximate the range of values of these parameters [2, 3], the optimal values, particularly for  $a$ ,  $A$ , and  $b$ , must be found individually for each system.

Before applying self-guided tomography to unknown qudits, we have examined different values for each of the hyperparameters to find their optimum values. To have comparable results, we pick one specific quantum state for a qutrit ( $d=3$ ) and always use the same starting point  $|\sigma_0\rangle$  for the algorithm. The resulting infidelities can be seen in Fig. S1. Our benchmarks for selecting the best coefficients have been the convergence of the infidelity, as well as the rate of convergence, i.e. achieving the smallest infidelities in the least number of iterations. In every graph, the green line is the optimum result, although the behavior for the selected values is very similar. For example, Fig. S1a shows no significant change between the orange, green and red line ( $a=5, 6$  and  $7$ ), with just the

blue line ( $a=1$ ) converging more slowly. The situation is similar for the green and red lines ( $b=0.1$  and  $1$ , respectively) in Fig. S1b; both converge at a comparable rate, and the orange and blue line ( $b=0.01$  and  $0.001$ ) with one and two orders of magnitude smaller values for  $b$ , respectively, converge very slowly. Fig. S1(c-e), showing the convergence results for  $s, t, A$ , respectively, further indicate the high robustness of these hyperparameters to large changes. Note, as self-guided tomography uses different random states in each iteration of each run, we expect slight deviations between consecutive measurements even for the same set of hyperparameters.

---

\* m.rambach@uq.edu.au

† m.romero@uq.edu.au

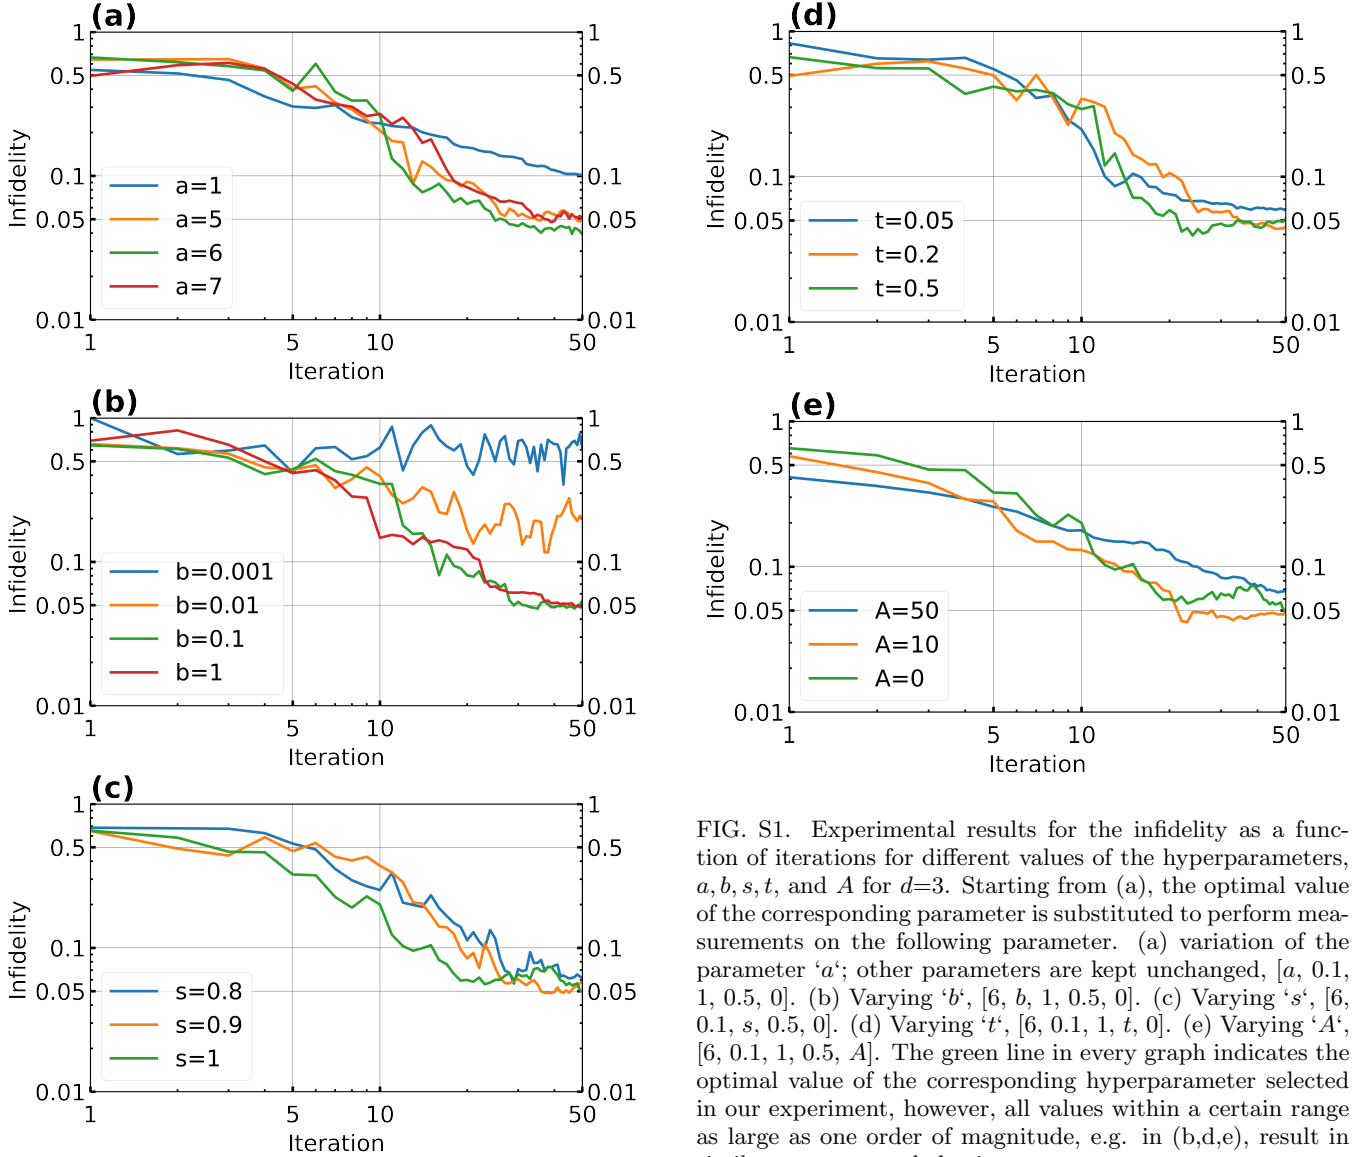

FIG. S1. Experimental results for the infidelity as a function of iterations for different values of the hyperparameters,  $a, b, s, t$ , and  $A$  for  $d=3$ . Starting from (a), the optimal value of the corresponding parameter is substituted to perform measurements on the following parameter. (a) variation of the parameter ‘ $a$ ’, other parameters are kept unchanged,  $[a, 0.1, 1, 0.5, 0]$ . (b) Varying ‘ $b$ ’,  $[6, b, 1, 0.5, 0]$ . (c) Varying ‘ $s$ ’,  $[6, 0.1, s, 0.5, 0]$ . (d) Varying ‘ $t$ ’,  $[6, 0.1, 1, t, 0]$ . (e) Varying ‘ $A$ ’,  $[6, 0.1, 1, 0.5, A]$ . The green line in every graph indicates the optimal value of the corresponding hyperparameter selected in our experiment, however, all values within a certain range as large as one order of magnitude, e.g. in (b,d,e), result in similar convergence behaviour.

## S2. EXPERIMENT DETAILS

We prepare and measure our quantum states using computer-generated holograms displayed on liquid-crystal spatial light modulators (SLM), see Fig. S2. We start with a weak coherent state from a highly attenuated CW laser at  $\sim 807$  nm in the fundamental Laguerre-Gauss mode  $|0,0\rangle$ . After the laser, a set of waveplates aligns the polarisation of the incoming light with the axis of the encoding SLM (eSLM) that is used to prepare the unknown quantum state  $|\psi\rangle$ . The reflected beam is focused towards an iris which filters out all higher diffraction orders excluding the first. A carefully aligned  $4f$ -lens setup—the diagonal beam path in Fig. S2—images the encoding SLM onto the measuring SLM (mSLM) where another hologram—corresponding to the state  $|\sigma\rangle$  being measured—is displayed. The imaging allows us to ef-

fectively quantify the overlap  $f(\sigma) = |\langle\sigma|\psi\rangle|^2$  via phase-flattening [4]. In every iteration, the measurement states  $|\sigma_{\pm}\rangle$  are chosen by the algorithm as described in Eqs.1 and 2 of the main text. After the mSLM, the photons are spatially filtered via an iris and a single-mode fibre to keep crosstalk between modes to a minimum. The mean photon number is  $|\alpha|^2 \sim 0.01$  and we detect  $\sim 10^5$  photons/s using a silicon avalanche photodiode detector with dark counts of  $\sim 300$  photons/s (Perkin-Elmer AQR-14), connected to a time tagging module (Swabian TT20).

## S3. CONSIDERATIONS ON THE TRUE ENCODED STATE

When estimating a quantum state with tomography, we have to take the quality of the state preparation into account. Assuming high fidelity state preparation, e.g. in

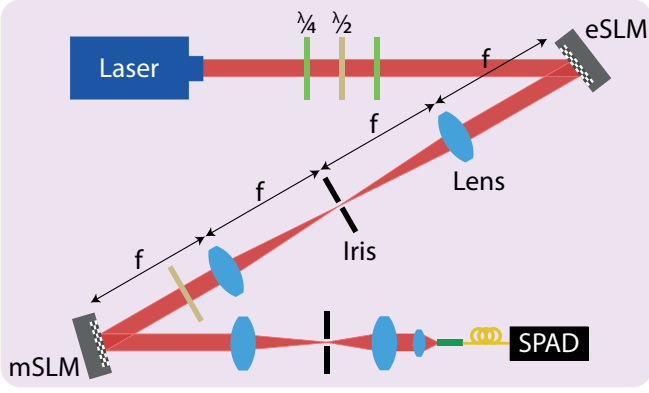

FIG. S2. Experimental realisation of self-guided tomography. The iris selects the first order from the eSLM. Lenses of focal length  $f$  are used in a  $4f$  arrangement to image the eSLM plane to a measurement SLM (mSLM) that displays the hologram for  $|\sigma_k\rangle$ . The combination of mSLM and the single mode fibre connected to a single photon avalanche detector (SPAD) allows us to infer the overlap between  $|\psi\rangle$  and  $|\sigma_k\rangle$ , which is then used to modify the measured state  $|\sigma_{k+1}\rangle$  in the next iteration.

ionic systems, the theoretically encoded state is very close to the actual prepared state. However, as the Hilbert space of the system grows, it becomes increasingly difficult to faithfully prepare the theoretical state. This will lead to lower fidelities when performing tomography, seemingly decreasing the achievable performance of your tomography algorithm.

To avoid this artificial decrease in fidelity, especially when approaching high values above 99%, we characterised the overlaps of multiple possible *true* states: the theoretically encoded state  $|\psi\rangle_{\text{th}}$ , the state found by long measurements of over-complete standard tomography  $|\psi\rangle_{\text{ST}}$  and the state found by self-guided tomography after a high number of iterations  $|\psi\rangle_{\text{SGT}}$ . The results can be found in Table S1. For the standard tomography, we increased the integration time from 1 to 10 seconds for each measurement, i.e.  $\sim 10$  million copies of the unknown state. For self-guided tomography, the algorithm uses 5, 2.5, and 4 times more iterations than in our results in the main article for the qutrit (500 iterations), ququint (500 iterations) and quvigint (2000 iterations), respectively, with the chosen number of iterations mainly limited by time constraints. Table S1 shows that the fidelity between the results from standard tomography and respectively  $|\psi\rangle_{\text{th}}$  and  $|\psi\rangle_{\text{SGT}}$  are the lowest, for both qutrit and ququint. This indicates that using  $|\psi\rangle_{\text{ST}}$  as your true state is a poor choice as expected by the susceptibility of standard tomography to all sources of error, e.g. mode-dependent losses where the efficiency of detecting different modes is not uniform. However, comparing  $|\psi\rangle_{\text{th}}$  and  $|\psi\rangle_{\text{SGT}}$  shows a high degree of overlap for all dimensions. We therefore chose the true state to be the experimentally found  $|\psi\rangle_{\text{SGT}}$ , as this avoids including preparation inaccuracies into the characterisation. Note

TABLE S1. Fidelities between the considered true states.  $|\psi\rangle_{\text{th}}$ , theoretically encoded state;  $|\psi\rangle_{\text{ST}}$ , state found by long measurements of over-complete standard tomography using  $\sim 10$  million copies of the unknown state per measurement;  $|\psi\rangle_{\text{SGT}}$ , state found by self-guided tomography after 500 (qutrit and ququint) or 2000 (quvigint) iterations of the algorithm. The overlap between the standard tomography results and respectively the theoretically encoded states or the self-guided tomography results is the lowest, hence it was not used as the true state. Comparing  $|\psi\rangle_{\text{th}}$  and  $|\psi\rangle_{\text{SGT}}$  on the other hand shows a high degree of overlap for all dimensions. In order to avoid including preparation inaccuracies we chose the experimentally found  $|\psi\rangle_{\text{SGT}}$  as the true state.

| Dimension |                            | $ \psi\rangle_{\text{SGT}}$ | $ \psi\rangle_{\text{ST}}$ |
|-----------|----------------------------|-----------------------------|----------------------------|
| 3         | $ \psi\rangle_{\text{th}}$ | $99.66^{+0.13}_{-0.19}$     | $95.8^{+0.1}_{-2.9}$       |
|           | $ \psi\rangle_{\text{ST}}$ | $96.3^{+1.0}_{-2.6}$        | -                          |
| 5         | $ \psi\rangle_{\text{th}}$ | $99.52^{+0.11}_{-0.26}$     | $95.3^{+1.4}_{-1.4}$       |
|           | $ \psi\rangle_{\text{ST}}$ | $96.2^{+1.6}_{-0.8}$        | -                          |
| 20        | $ \psi\rangle_{\text{th}}$ | $95.4^{+0.6}_{-3.8}$        | -                          |

that using  $|\psi\rangle_{\text{th}}$  as the true state still results in monotonically increasing (decreasing) fidelities (infidelities) and therefore arbitrary accurate state estimation, albeit at a lower rate.

#### S4. PREPARE-MEASURE CORRELATION MATRICES

The prepare-measure correlation matrix is a  $d \times d$  matrix which shows how well we can prepare and measure modes. The elements of the matrix are a measure for the overlap of the optical modes  $|\langle \sigma | \psi \rangle|^2$ , where  $|\psi\rangle$  is the prepared mode and  $|\sigma\rangle$  is the measured mode. Ideally, the matrix element will be high if we are preparing and measuring the same mode, and zero otherwise. Thus, the matrix shows the crosstalk between the orthogonal modes forming the basis set of our  $d$ -dimensional Hilbert space. We use transverse spatial modes of light as described by the Laguerre-Gaussian (LG) basis. To ascertain the accuracy of our measurements, we first experimentally derive the prepare-measure correlation coefficients for the states of the logical basis for each dimension  $d$ . It is important to ensure that the overlap between orthogonal modes is minimised.

The LG modes of light are prepared using two spatial light modulators (SLM) which encode the theoretical true state (encoding, eSLM) and measure the estimated state (measurement, mSLM). To measure each element of the prepare-measure correlation matrix, we prepare one of the eigenstates on the eSLM and measure it against all eigenstates on the mSLM. The maximum overlap is achieved when each spatial mode is projected onto itself resulting in a Gaussian beam shape which is then coupled

into a single mode fibre and further to a single photon detector that records the number of counts (see Fig. 2 in the main article).

To optimise the prepare-measure correlation matrix, the setup needs to be precisely aligned. Small degrees of misalignment in optical elements can result in significant overlap between orthogonal modes which appears as a non-zero off-diagonal correlation coefficient. We have measured the matrices for three different dimensions  $d=3, 5, 20$  as shown in Fig. S3 in the left (simulation) and right (experiment) column.

We would like to highlight that in the experimental results, the off-diagonal matrix elements show some overlap between nominally orthogonal modes. This overlap is not equally distributed over the matrix but rather favours adjacent modes before quickly tapering off for more distant states. This implies there are mode-dependent correlations and losses leading to a complex dependence of the experimental errors on the encoded/measured modes. To compare the experiment with simulations we introduce the visibility  $V$ . It is defined as the ratio of the sum of diagonal entries to the sum over all matrix elements, i.e.

$$V = \frac{\sum_{i=1}^d N_{ii}}{\sum_{i,j=1}^d N_{ij}} \quad (2)$$

where  $N_{ij}$  is the number of counts registered by the detector for encoded mode  $i$  and measured mode  $j$ . We reach a maximum experimental visibility of  $V=99.77\pm0.01\%$  in our experiment for  $d=3$ . Table. S2 shows the visibility values, which remain high for different dimensions.

To simulate our experimental results, we recreate the experimental values for dark counts ( $N\sim10^2-10^3$ ) and counting noise ( $\Delta N\sim10^2-10^3$ ) and introduce a random noise parameter to simulate all other noise sources. We then use the parameters to calculate average visibilities and tune the noise parameter to recreate the experimental value.

Unlike the experimental case, the simulated noise is uniformly distributed over all values  $N_{ij}$ . The mode dependent loss is different for each mode (superposition of modes) and largely depends on the efficacy of the phase-flattening. We did not implement these in the simulations and as a result, we expect some deviations between

the theoretical and experimental results of the prepare-measure correlation matrix, especially for higher  $d$  where modes with a higher mode number have less counts compared to the modes that have a lower mode number (see Fig S3c and f). This furthermore explains the slight discrepancies between simulations and experiments in self-guided tomography of higher  $d$  as well. Fortunately, the majority of the effect of mode-dependent loss is overcome by the self-guided tomography algorithm in our experiment as highlighted by the very small infidelities reported in the main paper.

TABLE S2. Experimental results for the visibilities of the prepare-measure correlation matrix for different dimensions given by Eq. 2. The uncertainties are calculated via error propagation of Poissonian counting noise.

| Dimension | Visibility         |
|-----------|--------------------|
| $d = 3$   | $99.77 \pm 0.01\%$ |
| $d = 5$   | $99.09 \pm 0.01\%$ |
| $d = 20$  | $97.64 \pm 0.01\%$ |

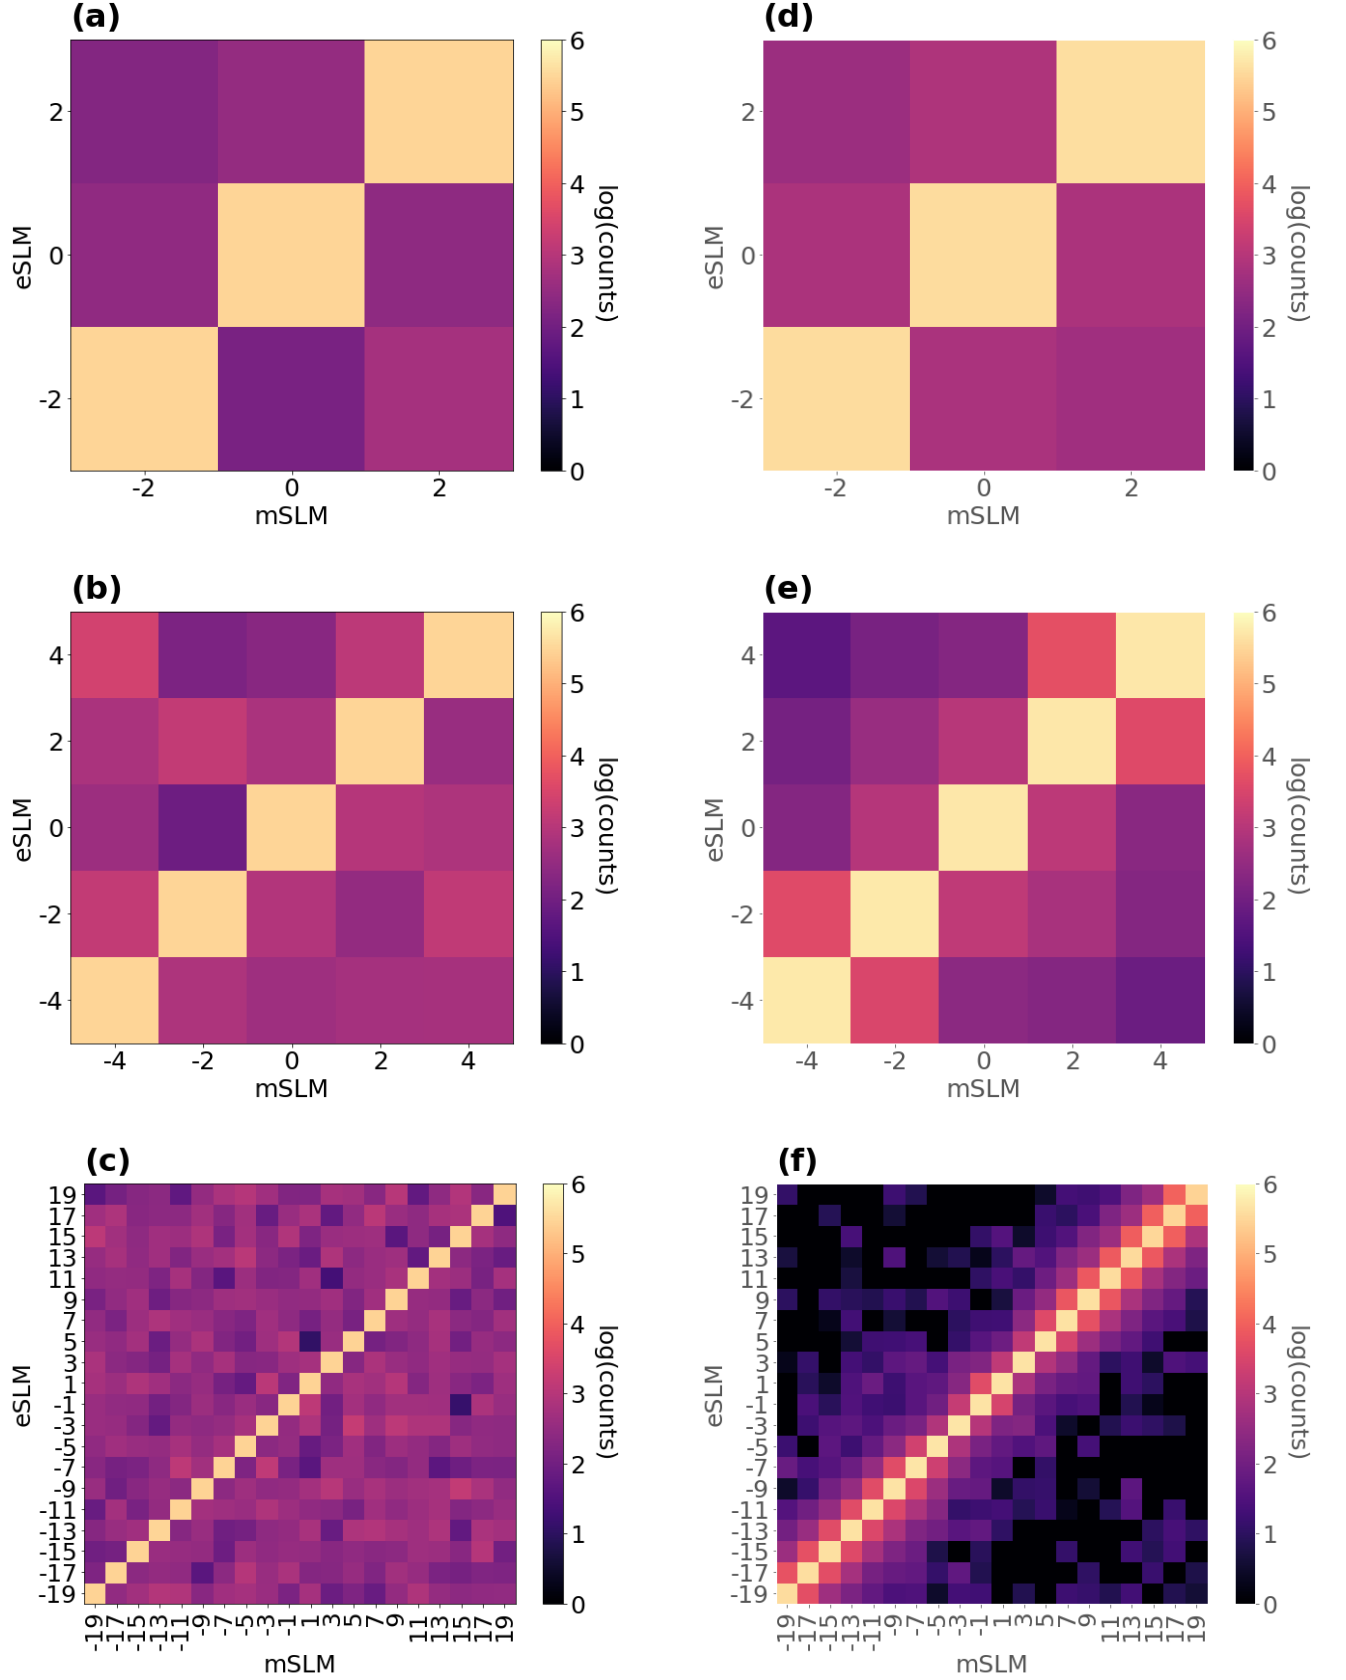

FIG. S3. Comparison of simulated (a-c) and experimental (d-e) prepare-measure correlation matrices for different dimensions  $d=3, 5, 20$ , respectively. Each element of the matrix is determined by registering the counts when encoding one mode on the eSLM (vertical axis, (we show only the azimuthal index for brevity) and another mode on the mSLM (horizontal axis). The nature of the experimental crosstalk, favouring adjacent modes especially visible for higher dimensions, is different from our simulations which show uniformly distributed noise. We used the set of Laguerre-Gaussian modes for our experiment, but any set of orthogonal modes will suffice.

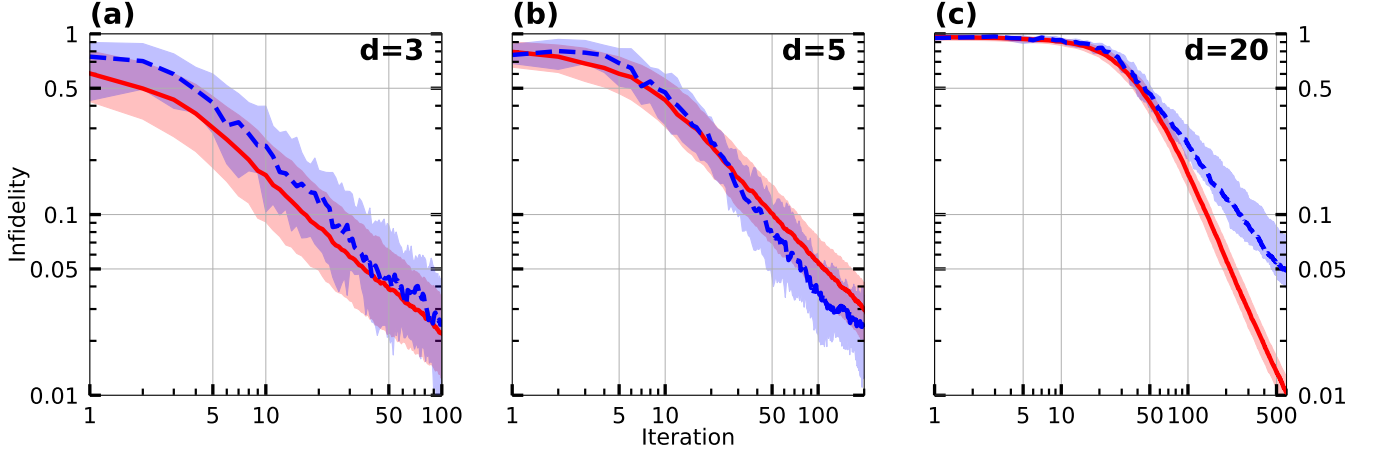

FIG. S4. Self-guided tomography in the presence of high statistical noise for (a) qutrit in 100 iterations, (b) ququint in 200 iterations, and (c) quvigint in 600 iterations. The dashed blue lines indicate the self-guided tomography results under the presence of high statistical noise, whereas the solid red lines are the equivalent simulations. The shaded area around each line surrounds the data 25% above and below the median. (Note: we have used the colour green for the experimental results in the main article for increased visibility).

#### S5. SELF-GUIDED TOMOGRAPHY WITH HIGH STATISTICAL NOISE: THEORY AND EXPERIMENT

We have implemented the self-guided tomography algorithm for low count rates to investigate its robustness to high statistical noise. The number of counts has been reduced to around 80 (per measurement) for  $d=3$  and 5, and around 1200 counts for  $d=20$ . The results are shown in Fig. S4. The graphs compare the experiment (dashed blue line) versus the equivalent simulated data (solid red line) for different dimensions. The experimental data shows continuing convergence to small infidelities, comparable with the theoretical results and highlighting the robustness of self-guided tomography to high statistical noise. While the infidelities for lower dimensions still overlap within the shaded uncertainty regions, we observe a small discrepancy between the experimental results and the simulated data for  $d=20$  for high iterations. We attribute this to an inadequate noise model of random but evenly distributed noise which fails to capture our experiment accurately. See Section S4 for further justification.

#### S6. ATMOSPHERIC TURBULENCE SIMULATIONS

We generate the phase holograms (or screens) to simulate atmospheric turbulence using Kolmogorov thin-film aberrations with an atmospheric turbulence strength of  $C_n^2 \sim 10^{-18} \text{ m}^{-2/3}$ . This strength relates to the Fried parameter  $r_0$ , the *coherence length of the phase aberrations*,

under assumption that  $C_n^2$  is constant via

$$r_0 = 0.185 \left( \frac{\lambda^2}{C_n^2 \cdot Z} \right)^{\frac{3}{5}}, \quad (3)$$

where  $\lambda$  is the wavelength and  $Z$  is the distance travelled through the atmosphere. The exponent and pre-factor stem from the Kolmogorov approximation of the turbulence. The actual value for  $C_n^2$  and  $r_0$  depend significantly on the location, e.g. inner city vs. country or the altitude, as well as the time of the day, weather phenomena like wind and of course the size of the photon mode.

The beam size in our experiment is fairly small (approx. 1 mm diameter) compared to usual real life turbulence experiments with transverse spatial modes (few to ten(s) of cm), e.g. in [5]. The important measure here is the ratio between the beam diameter  $D$  and the Fried parameter, in our case  $D/r_0 \ll 1$ . Hence, we are expecting only small detrimental effects on the mode shape. As an example, Malik and coworkers [6] showed that the capacity of an optical angular momentum communications channel for dimensions up to 11 remained largely unchanged for  $D/r_0 < 0.1$ , which is easily fulfilled in our experiment.

Our simulation generates a phase screen that is 150 by 150 pixels ( $\sim 1.4 \times 1.4 \text{ mm}$ ) in size and is overlapped with the original hologram of the measurement state at the center of the beam. Larger holograms take significantly more time (scaling approximately with total number of pixels  $\sim n_x \times n_y$ ) to simulate so we chose the minimum size that comfortably fits the beam diameter, hence avoiding any boundary effects. Fig. S5 depicts an example of a generated screen. In each iteration of self-guided tomography, one of these random screens is added to the original holograms for each measurement state  $|\sigma_{\pm, k}\rangle$ , respectively, and displayed on the SLM. Calculating a new

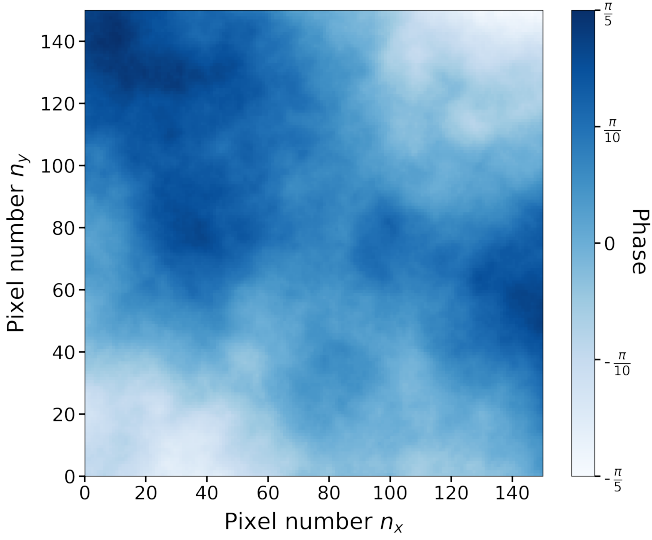

FIG. S5. Example of a phase screen to simulate atmospheric turbulence. The phase screen size on the SLM is 150 by 150 pixels ( $n_x \times n_y$ ), approximately 1.4 by 1.4 mm. The extrema of added phase are  $\sim \pm\pi/5$ , in white and dark blue. Similar phase screens are subsequently added to the unperturbed hologram of the quantum state on the measurement SLM.

random turbulence screen after every measurement simulates the always changing nature of the atmosphere.

### S7. COMPARISON BETWEEN SELF-GUIDED TOMOGRAPHY AND STANDARD TOMOGRAPHY

Table S3 compares qutrit and ququint self-guided tomography with standard tomography using a fixed amount of copies of the unknown state as well as theoretical and experimental results of self-guided tomography for all dimensions and scenarios under investigation. For the standard tomography, we applied maximum likelihood and root estimators [7] to measurements of the full set of mutually unbiased bases. To increase the precision of the standard tomography, we repeat the measurements ten times for a total of 120 (300) individual experiments, equal to 60 (150) iterations of self-guided tomography, for the qutrit (ququint).

We find that the simulated values for self-guided tomography overlap well with our experiments within their uncertainties. However, Table S3 also shows that independent of the dimension, we cannot surpass fidelities in the high 90% range using standard tomography. We attribute this limitation to mode-dependent losses of our system. Additionally, all achievable fidelities of standard tomography are lower than the values from self-guided tomography, which is not impacted by this limitation. This shows that self-guided tomography needs less resources than standard tomography to reach the same infidelity

and that the achieved fidelities keep increasing with the amount of iterations.

### S8. SELF-GUIDED TOMOGRAPHY ON MIXED STATES

Mixed states often arise in systems where there is less control of state preparation. To make self-guided tomography applicable in these situations we modified the algorithm to also work for mixed states. Although we tested the modified algorithm only for qutrit mixed states, the procedure is equally applicable to other dimensions—how the efficiency and accuracy scales with dimension will be an interesting future work.

The algorithm and its hyperparameters have to be slightly adjusted in order to work with mixed states: instead of estimating states, we have to estimate parametrised density matrices. For a qutrit, each mixed state is described by nine parameters, which are subsequently disturbed by a random step in each iteration  $k$ , either in the positive or negative direction. Step size and direction are defined analogously to the treatment of pure states. The parametrisation is then turned back into a density matrix  $\sigma_{\pm,k}$  for which we find the 3 eigenvalues  $v_{\pm,k}$  and eigenvectors  $\vec{w}_{\pm,k}$ . The (pure) eigenvectors are then displayed on the measurement SLM to find the probabilities  $p_{\pm,k,i} = n_{\pm,k,i}/N_{\pm,k}$ , with  $n_{\pm,k,i}$  the counts corresponding to the  $i^{\text{th}}$  eigenvector  $\vec{w}_{\pm,k,i}$  and  $N_{\pm} = \sum_i n_{\pm,k,i}$ , the total counts for all 3 eigenvectors. Finally, the algorithm calculates the  $j$ th component of the gradient at iteration  $k$  as

$$g_{kj} = \frac{f(\sigma_{+,k}) - f(\sigma_{-,k})}{2\beta_k \Delta_{kj}}. \quad (4)$$

However, in contrast to pure states, where  $f(\sigma_{\pm})$  are pseudo-normalised probabilities, here we use the quantum relative entropy

$$f(\sigma_{\pm,k}) = \sum_i p_{\pm,k,i} \log(v_{\pm,k,i}), \quad (5)$$

as our objective function. Any function that is quickly estimated from measurements and optimised when  $\sigma$  is the true state is suitable for self-guided tomography. Note that not every distance measure will work. Mixed-state fidelity, for example, would require full tomography to estimate, clearly defeating the purpose.

The density matrix of the mixed state is implemented in the form

$$\rho = \begin{pmatrix} p_1 & 0 & 0 \\ 0 & p_2 & 0 \\ 0 & 0 & p_3 \end{pmatrix}, \quad (6)$$

where  $\sum_m p_m = 1$ . As we generate highly pure states in our experiment, the mixture is introduced artificially. We realise  $\rho$  by picking a random state of the logical basis ( $|0\rangle, |1\rangle, |2\rangle$ ), based on a biased coin flip with probabilities  $p_i$ , and displaying it on the encoding SLM between

TABLE S3. Comparison of self-guided tomography (SGT) with standard tomography (ST). The amount of iterations in self-guided tomography are chosen adequately to the amount of measurements in standard tomography (for  $d=3, 5$ ) and the minimal necessary measurements for over-complete tomography [8] for the quvigit ( $\sim 800$ , i.e. 400 iterations). All values are the medians over the number of investigated states and the uncertainties are chosen to cover the interquartile ranges (median  $\pm 25\%$ ). *sim*, simulations with 1000 random states; *exp*, experiments with 50 and 20 random states for  $d=3, 5$  and  $d=20$ , respectively. Photon numbers for *low* and *high statistical noise* as well as a description of the *turbulence* can be found in the main article.

| Iterations | Qutrit, d = 3                           |                                         |                                      | Quqint, d = 5                           |                                         |                                      | Quvigit, d = 20                         |                                      |  |
|------------|-----------------------------------------|-----------------------------------------|--------------------------------------|-----------------------------------------|-----------------------------------------|--------------------------------------|-----------------------------------------|--------------------------------------|--|
|            | Self-guided                             |                                         | Standard                             | Self-guided                             |                                         | Standard                             | Self-guided                             |                                      |  |
|            | 60                                      |                                         |                                      | 150                                     |                                         |                                      | 400                                     |                                      |  |
|            | sim                                     | exp                                     |                                      | sim                                     | exp                                     |                                      | sim                                     | exp                                  |  |
| Low noise  | 99.81 <sup>+0.12</sup> <sub>-0.25</sub> | 99.77 <sup>+0.10</sup> <sub>-0.39</sub> | 96.3 <sup>+1.0</sup> <sub>-2.6</sub> | 99.72 <sup>+0.11</sup> <sub>-0.20</sub> | 99.82 <sup>+0.09</sup> <sub>-0.11</sub> | 97.4 <sup>+0.9</sup> <sub>-1.5</sub> | 98.80 <sup>+0.25</sup> <sub>-0.31</sub> | 97.9 <sup>+0.3</sup> <sub>-0.8</sub> |  |
| High noise | 96.6 <sup>+1.4</sup> <sub>-2.2</sub>    | 96.4 <sup>+1.3</sup> <sub>-2.5</sub>    | 95.5 <sup>+1.6</sup> <sub>-2.6</sub> | 96.2 <sup>+1.2</sup> <sub>-1.6</sub>    | 97.1 <sup>+1.0</sup> <sub>-1.2</sub>    | 95.6 <sup>+1.4</sup> <sub>-1.7</sub> | 98.11 <sup>+0.37</sup> <sub>-0.40</sub> | 93.5 <sup>+0.8</sup> <sub>-3.8</sub> |  |
| Turbulence | -                                       | 99.13 <sup>+0.49</sup> <sub>-1.49</sub> | 95.3 <sup>+1.9</sup> <sub>-2.9</sub> | -                                       | 98.94 <sup>+0.52</sup> <sub>-0.55</sub> | 95.9 <sup>+1.7</sup> <sub>-1.0</sub> | -                                       | 95.0 <sup>+1.4</sup> <sub>-2.8</sub> |  |

every measurement. We satisfactorily approximate the mixed state after several coin flips, typically after 50 flips, i.e. 25 iterations. Similar to the case of pure states, we simulated the performance of various hyperparameters and chose the ones that work best for our experiment.

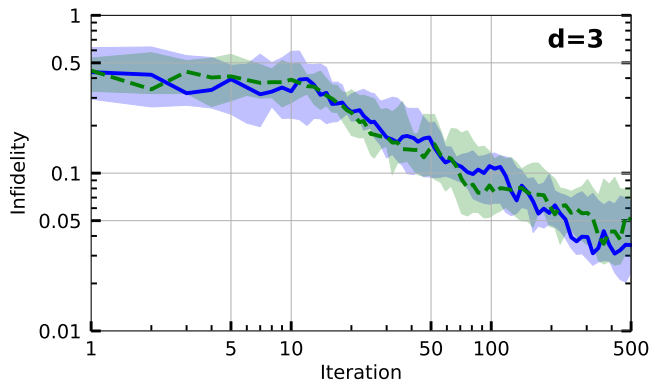

FIG. S6. Self-guided tomography on qutrit mixed states for low (solid blue) and high (dashed green) statistical noise. The lines are the median performance, while the shaded regions are bound by the upper and lower quartile of the infidelities,  $(50 \pm 25)\%$ .

Fig. S6 shows the results for low (blue solid) and high (green dashed) statistical noise, i.e. total counts  $N_{\pm}$  around 800000 and 800, respectively. We encoded 20 randomly chosen mixed states with purities  $P \equiv \text{Tr}(\rho^2)$  between 0.34 and 0.88 and performed 500 iterations of self-guided tomography. The average fidelities ( $=1 - \text{infidelity}$ ) are  $96.5 \pm 3.1\%$  ( $88.9 \pm 5.2\%$ ) after 500 (100) iterations in the low noise case, and  $94.9 \pm 2.2\%$  ( $91.6 \pm 3.3\%$ ) for high statistical noise. The values are slightly lower than the theoretically expected 99.1% (93%) for both high and low noise after 500 (100) iterations. However, this is to be expected as we need to accumulate statistics first in order to faithfully encode a mixed state in our experiment. More importantly, and analogue to the pure state performance, the straight line asymptotic behaviour highlights the expected power law relationship between infidelity and number of iterations. We believe that the algorithm will perform as theoretically expected for mixed states in other systems where the mixture occurs naturally. Finally, the adapted algorithm seems, to a certain degree, more robust to high statistical noise, theoretically with a fidelity as high as 96.5% for an average of  $N_{\pm}=10$  total counts and in practise as highlighted by the overlap of the two traces in Fig. S6. This would be make a compelling path for further investigations.

[1] C. Ferrie, Self-guided quantum tomography, Phys. Rev. Lett. **113**, 2 (2014).  
[2] J. C. Spall, Multivariate stochastic approximation using a simultaneous perturbation gradient approximation, IEEE Transactions on Automatic Control **37**, 332 (1992).  
[3] P. Sadegh and J. C. Spall, Correction to "optimal random perturbations for stochastic approximation using a simultaneous perturbation gradient approximation", IEEE Transactions on Automatic Control **44**, 231 (1999).  
[4] A. Mair, A. Vaziri, G. Weihs, and A. Zeilinger, Entanglement of the orbital angular momentum states of photons,

Nature **412**, 313 (2001).  
[5] M. Krenn, R. Fickler, M. Fink, J. Handsteiner, M. Malik, T. Scheidl, R. Ursin, and A. Zeilinger, Communication with spatially modulated light through turbulent air across Vienna, New J. Phys. **16** (2014).  
[6] M. Malik, M. O'Sullivan, B. Rodenburg, M. Mirhosseini, J. Leach, M. P. J. Lavery, M. J. Padgett, and R. W. Boyd, Influence of atmospheric turbulence on optical communications using orbital angular momentum for encoding, Opt. Express **20**, 13195 (2012).  
[7] Y. I. Bogdanov, Unified statistical method for reconstruct-

- ing quantum states by purification, J. Exp. Theor. Phys. **108**, 928 (2009).
- [8] N. K. Langford, R. B. Dalton, M. D. Harvey, J. L. O'Brien, G. J. Pryde, A. Gilchrist, S. D. Bartlett, and A. G. White, Measuring entangled qutrits and their use for quantum bit commitment, Phys. Rev. Lett. **93**, 1 (2004).
